# Supplementary material for: Scaling Large-scale GNN Training to Thousands of Processors on CPU-based Supercomputers
Source: arXiv:2411.16025 source file (2025-05-26)
Supplement: Supplementary file 1 [file 8-appendix.tex]

\appendix

\section{proofs of Lemmas}

\subsection{Lemma 1}
%\begin{lemma}
\begin{proof}
We perform Taylor expansion for $\nabla \widetilde {\mathcal L}(W_t)$:

\begin{equation}
\small
\begin{aligned}
& \widetilde g_t(\mathbf{w}_{t+1}) = \widetilde {\mathcal L}(\mathbf{w}_t-\eta \mathbf{g}_t) + \eta(\mathbf{g}_t - \mathbf{\tilde{g}}_t)^T \widetilde {\mathcal L}(\mathbf{w}_t - \eta \mathbf{g}_t) \\
& + \frac{1}{2}\eta^2 (\mathbf{g}_t - \mathbf{\tilde{g}}_t)^T \nabla^2 \mathcal{L}(\mathbf{\epsilon}_t)(\mathbf{g}_t - \mathbf{\tilde{g}}_t)
\end{aligned}
\label{eq:lemma1:one}
\end{equation}

From Assumption (b) $\mathbb{E}[\mathbf{\tilde{g}}_t] = \mathbf{g}_t$. By substituting $\mathbb{E}[\mathbf{\tilde{g}}_t]$ in Eqn.~\ref{eq:lemma1:one}, we have:

\begin{equation}\label{Eq:first}
\small
\begin{aligned}
& \mathbb{E}[\widetilde {\mathcal L}(\mathbf{w}_{t+1})]  \leq \mathbb{E}[\widetilde {\mathcal L}(\mathbf{w}_t-\eta \mathbf{g}_t) \\
& + \eta(\mathbf{g}_t - \mathbf{\tilde{g}}_t)^T \nabla \widetilde {\mathcal L}(\mathbf{w}_t - \eta \mathbf{g}_t) \\
& + \frac{1}{2}\eta^2 \rho||\mathbf{g}_t - \mathbf{\tilde{g}}_t||^2] \\
& \leq \mathbb{E}[\widetilde {\mathcal L}(\mathbf{w}_t-\eta \mathbf{g}_t)] + \frac{1}{2}\eta^2\rho K^2
\end{aligned}
\end{equation}

where the left-hand side of the inequality is an attribute of Assumption (a), i.e. Lipschitz continuity, and the right-hand side of the inequality is attributed to Assumption (c) on the boundness of the variance of the approximate gradient. We apply the Taylor expansion in Eqn.~\ref{Eq:first} to $\widetilde {\mathcal L}(\mathbf{w}_t-\eta \mathbf{g}_t)$, and rewrite Eqn.~\ref{Eq:first} as:
\begin{equation}
    \begin{aligned}
    & (\eta - \frac{1}{2}\eta^2 \rho)\mathbb{E}[||\nabla \widetilde {\mathcal L}(\mathbf{w}_t)||^2] \leq \mathbb{E}[\widetilde {\mathcal L}(\mathbf{w}_t)] - \mathbb{E}[\widetilde {\mathcal L}(\mathbf{w}_{t+1})] \\
    & + \frac{1}{2}\eta^2 \rho K^2
    \end{aligned}
\end{equation}
since all assumptions are predicated on the existence of a global minimum, summing the global minimum over the epochs T we train bounds the convergence variance as follows:

\begin{equation}
\small
    \begin{aligned}
    \frac{\sum_{t=1}^T\mathbb{E}[||\nabla \widetilde {\mathcal L}(\mathbf{w}_t)||^2]}{T} \leq \frac{2(\widetilde {\mathcal L}(\mathbf{w_1})-\widetilde {\mathcal L}^{\ast})}{T(2\eta - \rho\eta^2)} + \frac{\eta \rho}{2-\eta \rho} \cdot  K^2
    \end{aligned}
\end{equation}
\end{proof}

\subsection{Lemma 2}
%\begin{lemma}
\begin{proof}
With a fixed int2 model quantization variance $\frac{\partial \mathcal{L}}{\partial \mathbf{\tilde{W}}^l}$ for layer $l$, and the original FP32 precision counterpart as $\frac{\partial \mathcal{L}}{\partial \mathbf{W}^l}$. The quantization variance quantization variance $\frac{\partial \mathcal{L}}{\partial \mathbf{\tilde{W}}^l}$ for the forward path (at layer $l$) can be written as:

\begin{equation}
\small
\begin{aligned}
    & \frac{\partial \mathcal{L}}{\partial \mathbf{\tilde{W}}^l} =  \sum_v^{|V|}\sigma'(\cdot) \odot \frac{\partial \mathcal{L}}{\partial h_v^l}(\sum_{u}^{\{v\} \cup N(v)} \alpha_{u,v}h_u^{l-1})^T \\
    & = \sum_v^{|V|}\sigma'(\cdot) \odot (\sum_{u}^{\{v\} \cup N_{L}(v)}\alpha_{u,v}\frac{\partial \mathcal{L}}{\partial h_u^l} + \sum_{k}^{N_{R}(v)}\alpha_{k,v}\frac{\partial \mathcal{L}}{\partial \hat{h}_{k_2}^l}) \cdot \\ & (\sum_{u}^{\{v\} \cup N_{L}(v)}\alpha_{u,v}h_u^{l-1} + \sum_{k}^{N_{R}(v)}\alpha_{k,v}\hat{h}_{k_2}^{l-1})^T
\end{aligned}
\end{equation}

Where $h_u^l$ is the weighed summation form of embedding generation used commonly in GCNs~\cite{kipf2016semi} when adjusted for int2 quantization. Treating the message passing for the forward pass as independent from the backward pass, and considering that the the summation form $h_u^l$  to be unbiased and variance bounded, per Theorem 1 from~\cite{wan2023adaptive}, the expectation of $\frac{\partial \mathcal{L}}{\partial \mathbf{\tilde{W}}^l}$ can be expressed as:

\begin{equation}
\small
    \begin{aligned}
        & \mathbb{E}[\frac{\partial \mathcal{L}}{\partial \mathbf{\tilde{W}}^l}] = \sum_v^{|V|}\sigma'(\cdot) \odot (\sum_{u}^{\{v\} \cup N_{L}(v)}\alpha_{u,v}\frac{\partial \mathcal{L}}{\partial h_u^l} \\
    & + \sum_{k}^{N_{R}(v)}\alpha_{k,v}\mathbb{E}[\frac{\partial \mathcal{L}}{\partial \hat{h}_{k_2}^l}])(\sum_{u}^{\{v\} \cup N_{L}(v)}\alpha_{u,v}h_u^{l-1} \\
    & + \sum_{k}^{N_{R}(v)}\alpha_{k,v}\mathbb{E}[\hat{h}_{k_2}^{l-1}])^T \\
    \end{aligned}
\end{equation}

The variance $\mathbb{V}ar$ is defined as: 

\begin{equation}
\small
    \begin{aligned}
        & \mathbb{V}ar[\frac{\partial \mathcal{L}}{\partial \mathbf{\tilde{W}}^l}] = \sum_v^{|V|}\mathbb{V}ar[\frac{\partial \mathcal{L}}{\partial h_v^l}(\sum_u^{\{v\} \cup N(v)}\alpha_{u,v}h_u^{l-1})^T] \\
        & = \sum_v^{|V|} \mathbb{E}[(\frac{\partial \mathcal{L}}{\partial h_v^l})^2]\mathbb{E}[(\sum_u^{\{v\} \cup N(v)}\alpha_{u,v}h_u^{l-1})^2]^T \\
        & - \mathbb{E}[\frac{\partial \mathcal{L}}{\partial h_v^l}]^2\mathbb{E}[(\sum_u^{\{v\} \cup N(v)}\alpha_{u,v}h_u^{l-1})^T]^2 \\
    \end{aligned}
\end{equation}

Using Theorem 1 from~\cite{wan2023adaptive}, we have:
\begin{equation}\label{proof:upper_bound}
\small
    \begin{aligned}
        & \mathbb{V}ar[\frac{\partial \mathcal{L}}{\partial \mathbf{\tilde{W}}^l}] \leq \sum_v^{|V|} (\sum_k^{N_{R}(v)}\alpha^2_{k,v}\frac{D_k^l \cdot (S_{k_2}^l)^2}{6}) \\
         & \cdot (\sum_k^{N_{R}(v)}\alpha^2_{k,v}\frac{D_k^{l-1} \cdot (S_{k_2}^{l-1})^2}{6}) + M^2 \sum_k^{N_R(V)}\alpha^2_{k,v} \frac{D_k^{l}(S_{k_2}^{l})^2}{6} \\
         & + N^2 \sum_k^{N_R(v)}\alpha^2_{k,v} \frac{D_k^{l-1}(S_{k_2}^{l-1})^2}{6})
    \end{aligned}
\end{equation}

The gradient variance upper bound $K^l$ in layer $l$ substituted for the gradient variance upper bound in Eqn.~\ref{proof:upper_bound} becomes:
\begin{equation}
\small
    \begin{aligned}
          & K^l = \sum_v^{|V|}(\sum_{k_1}^{N_R(v)}\sum_{k_2}^{N_R(v)}\alpha^2_{k_1,v}\alpha^2_{k_2,v} \frac{D_{k_1}^{l-1}D_{k_2}^l(S_{k_{1_2}}^{l-1}S_{k_{2_2}}^l)^2}{6}\\
         &+ M^2 \sum_k^{N_R(v)}\alpha^2_{k,v} \frac{D_k^{l}(S_{k_2}^{l})^2}{6}
         + N^2 \sum_k^{N_R(v)}\alpha^2_{k,v} \frac{D_k^{l-1}(S_{k_2}^{l-1})^2}{6})
    \end{aligned}
\end{equation}

\end{proof}
