# Supplementary material for: Scaling Large-scale GNN Training to Thousands of Processors on CPU-based Supercomputers
Source: arXiv:2411.16025 source file (2025-05-26)
Supplement: Supplementary file 2 [file appendix.tex]

\section{Experiments setup}
%%%%%%%%%%%%%%%%%%%%%%%
 \begin{table}
      \caption{The graph datasets used in experiments.}        
      \small
      \centering
      %\vspace{-10pt}
      \resizebox{\linewidth}{!}{
          \begin{tabular}{ |l|c|c|c|c| }
          \hline
          \bf{Datasets} & \bf{\#Vertex} & \bf{\#Edges} & \bf{\#Feat} & \bf{\#Class} \\
          \hline
          \textsf{Ogbn-arxiv} & 169,343 & 1,166,243 & 128 & 40 \\
          % \hline
          \textsf{Reddit} & 232,965 & 114,615,892 & 602 & 41 \\
          % \hline
          \textsf{Ogbn-products} & 2,449,029 & 61,859,140 & 100 & 47 \\
          % \hline
          \textsf{Proteins} & 8,745,542 & 1,309,240,502 & 128 & 256 \\
          % \hline
          \textsf{Ogbn-papers100M} & 111,059,956 & 1,615,685,872 & 128 & 172 \\
          % \hline
          \zhuang{\textsf{Ogb-lsc-mag240M$^{*}$}} & 121,751,666 & 2,593,241,212 & 768 & 153 \\
          \textsf{UK-2007-05} & 105,896,555 & 3,738,733,648 & 128 & 172 \\
          % \hline
          % Ogbn-papers100M & 111,059,956 & 1,615,685,872 & 128 & 72 \\
          \hline
          \multicolumn{4}{l}{$^{*}$We extract the undirected homogeneous papers citation graph.}
           \end{tabular}  
        }
       \label{table/experiment:dataset} 
\end{table}     
%%%%%%%%%%%%%%%%%%%%%%%%%
\textbf{Hardware.} 
ABCI's compute nodes are connected with InfiniBand and contain two Intel Xeon Gold 6148 CPUs running at 2.4 GHz, each with 20 cores, 384GB of DDR4 memory, and a theoretical peak bandwidth to DRAM of 128GB/s. On the other hand, Fugaku's compute nodes are connected via the Tofu 6D torus network and feature Fujitsu ARM A64FX processors. These processors have 48 cores running at 2.0 GHz, organized into 4 CMGs with each CMG containing 12 cores. Fugaku is equipped with HBM2 memory, providing a capacity of 32GB and a memory bandwidth of up to 1024GB/s.

\textbf{Software.} We use the following: Pytorch v1.10.0, Pytorch Geometric v2.0.4, Pytorch Sparse v0.6.13, and Pytorch Scatter v2.0.9.
On ABCI, 
% we compiled our code using GCC 8.3.1 with the following options: "-O3 -fopenmp -mavx512f." Additionally, for MPI communication, 
we use Intel oneCCL v1.10.0 as the backend for the torch.distributed package on Intel platforms. We use one MPI rank per one Intel CPU.
On Fugaku, 
% we compiled our code using the Fujitsu compiler version 1.3.33 with options: " -Kfast -Nclang -Kopenmp." For MPI communication, 
we use the built-in Fujitsu MPI as the backend for the torch.distributed package. We use one MPI rank per one CMG on A64FX.

\section{Ablation study on multiple NUMA nodes}
\begin{figure}
    \centering
    \includegraphics[width=0.985\linewidth]{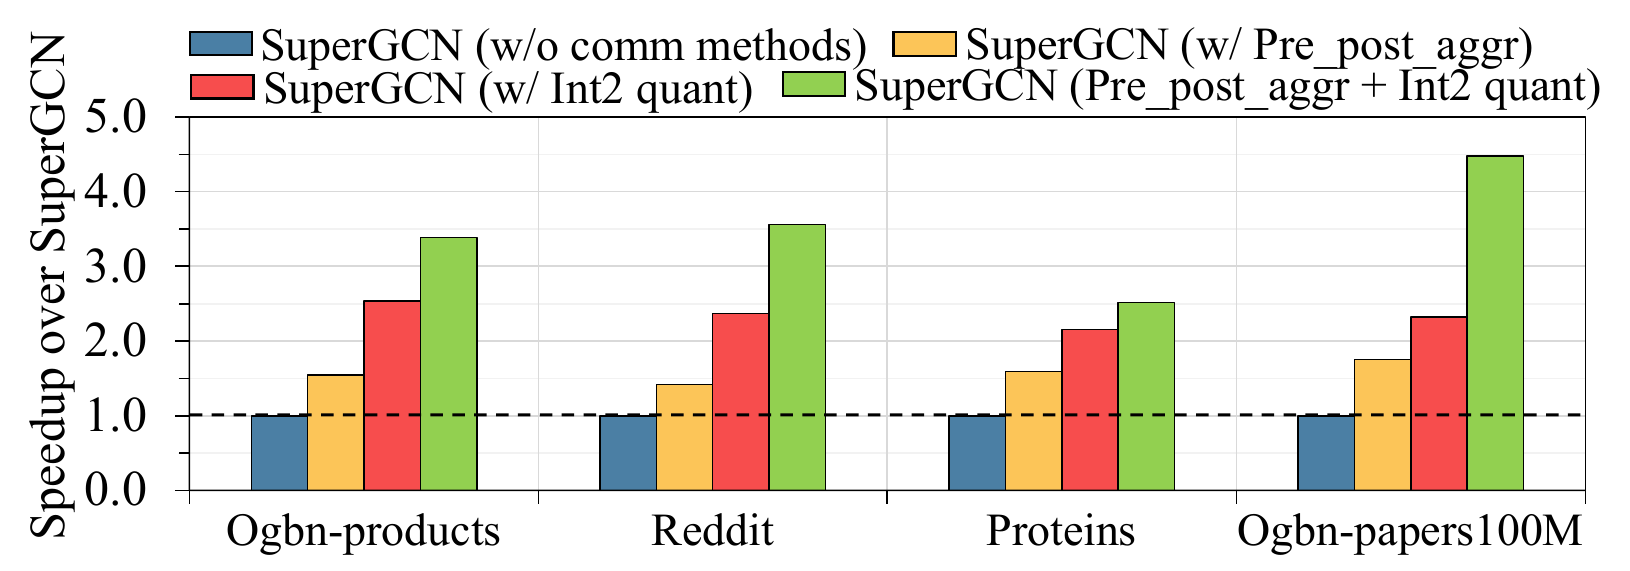}
    \caption{Ablation study of different datasets on ABCI (256 MPI processes).}
    \label{fig/experiment:ablation_study_256}
\end{figure}

To evaluate the performance benefits of each proposed method, we conducted an ablation study on different datasets using ABCI with 256 CPUs. The results are shown in Fig.~\ref{fig/experiment:ablation_study_256}. In all datasets, compared with the vanilla method, the pre-post-aggregation methods achieve a speedup ranging from 1.4x to 1.8x, as they significantly decrease communication volume. The random bits quantization method also gains a speedup ranging from 2.4x to 2.8x, since it has a similar impact on performance by reducing communication volume while scaling the proposed system to numerous CPUs. Consequently, by combining these two proposed methods, a higher speedup is achieved on both 4 datasets.

\section{proof}
The proof of Theorem 1:

Based on the assumption (a), we have:
{\footnotesize
$$
L(W_{t+1}) \leq L(W_{t}) + \langle \nabla L(W_{t}), W_{t+1} - W_{t} \rangle + \frac{\rho}{2} \lVert W_{t+1} - W_{t} \rVert_2^2
$$
}
then plugging $W_{t+1} = W_{t} - \eta \cdot \nabla \widetilde {\mathcal L} (W_t)$ into it:
{
\footnotesize
$$
L(W_{i+1}) \leq L(W_{i}) - \eta \cdot \langle {\mathcal L} (W_t),  \nabla \widetilde {\mathcal L} (W_t) \rangle + \frac{\rho\eta^2}{2} \lVert  \nabla \widetilde {\mathcal L} (W_t) \rVert_2^2
$$
}
let $\delta_t = \nabla L (W_t) - \nabla \widetilde L (W_t)$
{\footnotesize
$$
L(W_{i+1}) \leq L(W_{i}) - \eta \cdot \lVert \nabla {\mathcal L} (W_t) \rVert_2^2 + \eta \cdot \langle \nabla {\mathcal L} (W_t), \delta_t \rangle 
$$
$$
+ \frac{\rho\eta^2}{2}[\lVert  \nabla {\mathcal L} (W_t) \rVert_2^2 + \rVert \delta_t \rVert_2^2 - 2 \langle \nabla {\mathcal L} (W_t), \delta_t \rangle]
$$
$$
\leq {\mathcal L} (W_t) - 
$$
}
